# Supplementary material for: Hyperbolic Neural Networks++
Source: arXiv:2006.08210 source file (2021-03-17)
Supplement: Supplementary file 1 [file centroid_coaddition.tex]

\subsection{The reasonability of the generalization of the Möbius coaddition}
\label{subsec:reasonability_coadd_centroid}
We previously described that the novel operator $\gmcplus{N}{i=1}{\bm{b}_i, \nu_i}$ in Equation \ref{eq:poincare_weighted_centroid} for arbitrary points $\{\bm{b}_i\in\mathspace{B}{n}{c}\}^N_{i=1}$ and scalar weights $\{\nu_i\in\mathspace{R}{}{}\}^N_{i=1}$ can be contracted into the Möbius coaddition in certain cases in which there are two operands and the weights have the same positive values, which indicates that two operands are equally summed:
\begin{align}
    \label{eq:poincare_centroid_and_coaddition_indication}
    \gmcplus{2}{i=1}{\bm{b}_i, \nu}
    =2\frac{\sum^2_{i=1}\nu\frac{\bm{b}_i}{1-c\pnorm{\bm{b}_i}{2}{}}}{\sum^2_{i=1}\nu\frac{1+c\pnorm{\bm{b}_i}{2}{}}{1-c\pnorm{\bm{b}_i}{2}{}}}
    = \frac{\sbrakets{1-c\pnorm{\bm{b}_2}{2}{}}\bm{b}_1+\sbrakets{1-c\pnorm{\bm{b}_1}{2}{}}\bm{b}_2}{1-c^2\pnorm{\bm{b}_1}{2}{}\pnorm{\bm{b}_2}{2}{}}
    =\bm{b}_1\mcplus\bm{b}_2
    \text{.}
\end{align}
In this subsection, we show an intuitive way to naturally extend the expression of the Möbius coaddition that also matches our proposed operator.

From Equation \ref{eq:gamma_mobius_coaddition}, we can expand the equation of the Möbius coaddition such that it can be clearly seen as a commutative binary operation for $\bm{b}_1,\bm{b}_2\in\mathspace{B}{n}{c}$:
\begin{align}
    \bm{b}_1\mcplus\bm{b}_2 = 
    \frac{\gamma^2_{\bm{b}_1}\bm{b}_1+\gamma^2_{\bm{b}_2}\bm{b}_2}{\gamma^2_{\bm{b}_1}+\gamma^2_{\bm{b}_2}-1}
    =
    \frac{\sum^2_{i=1}\gamma^2_{\bm{b}_i}\bm{b}_i}{\sum^2_{i=1}\sbrakets{\gamma^2_{\bm{b}_i}-\frac{1}{2}}}
    \text{.}
\end{align}
As a commutative multinary operation for $\{\bm{b}_i\in\mathspace{B}{n}{c}\}^N_{i=1}$, we can naturally increase the number of additive operands in this equation as follows:
\begin{align}
    \frac{\sum^N_{i=1}\gamma^2_{\bm{b}_i}\bm{b}_i}{\sum^N_{i=1}\sbrakets{\gamma^2_{\bm{b}_i}-\frac{1}{2}}}
    \text{.}
\end{align}
Moreover, introducing scalar weights $\{\nu_i\in\mathspace{R}{}{}\}^N_{i=1}$ as the indicators of the dominance of each point $\bm{b}_i$ to the total summation, and regarding any negative weight as an additive inverse operation, we can further generalize this equation as follows:
\begin{align}
    \frac{\sum^N_{i=1}|\nu_i|\,\,\gamma^2_{\bm{b}_i}\mbrakets{\sign\sbrakets{\nu_i}\bm{b}_i}}{\sum^N_{i=1}|\nu_i|\sbrakets{\gamma^2_{\sign(\nu_i)\bm{b}_i}-\frac{1}{2}}}
    =
    \frac{\sum^N_{i=1}\nu_i\gamma^2_{\bm{b}_i}\bm{b}_i}{\sum^N_{i=1}|\nu_i|\sbrakets{\gamma^2_{\bm{b}_i}-\frac{1}{2}}}
    \text{,}
\end{align}
which exactly matches our proposed operator as a generalized Möbius coaddition:
\begin{align}
    \frac{\sum^N_{i=1}\nu_i\gamma^2_{\bm{b}_i}\bm{b}_i}{\sum^N_{i=1}|\nu_i|\sbrakets{\gamma^2_{\bm{b}_i}-\frac{1}{2}}}
    =\frac{\sum^N_{i=1}\nu_i\frac{\bm{b}_i}{1-c\pnorm{\bm{b}_i}{2}{}}}{\frac{1}{2}\sum^N_{i=1}|\nu_i|\frac{1+c\pnorm{\bm{b}_i}{2}{}}{1-c\pnorm{\bm{b}_i}{2}{}}}
    =\gmcplus{N}{i=1}{\bm{b}_i, \nu_i}
    \text{.}
\end{align}
